# Supplementary material for: Fast Kernelized Correlation Filters without Boundary Effect
Source: arXiv:1806.06406 source file (2020-09-23)
Supplement: Supplementary file 2 [file HSKCF_without_BE__Supplementary_Material___NIPS2018_.pdf]

---

# Supplementary Material

## High Speed Kernelized Correlation Filters without Boundary Effect

---

Ming TANG, Linyu ZHENG, Bin YU, Jinqiao WANG

University of Chinese Academy of Sciences

National Lab of Pattern Recognition, Institute of Automation, CAS, Beijing 100190, China

### Abstract

This supplementary material contains three parts. 1) Illustrations of Algorithm 2, CCIM. 2) Mathematical proof of the correctness of CCIM. 3) Other experimental results on popular data sets.

## 1 Notation

Let  $\diamond$  and  $\cdot$  be the correlation operator and dot product, respectively,  $\mathbf{H}((a_1, b_1), (a_2, b_2))$  be the sub-matrix of matrix  $\mathbf{H}$  with  $(a_1, b_1)$  and  $(a_2, b_2)$  as its top left and down right corner subscripts, respectively, and  $H_{a,b}$  be an element of matrix  $\mathbf{H}$ .

## 2 Illustration of Algorithm 2 (CCIM)

Let two images be

$$\mathbf{X}^{0,0} = \begin{bmatrix} 1 & 2 & 3 \\ 4 & 5 & 6 \\ 7 & 8 & 9 \end{bmatrix} \quad \text{and} \quad \mathbf{Z} = \begin{bmatrix} a & b & c & d & e \\ f & g & h & i & j \\ k & l & m & n & o \\ p & q & r & s & t \\ u & w & x & y & z \end{bmatrix},$$

respectively, where the numbers in  $\mathbf{X}^{0,0}$  indicate the elements of  $\mathbf{X}^{0,0}$ , rather than the elements' real feature values.  $\mathbf{X}^{0,0}$  and  $\mathbf{Z}$  are called base correlation filters and signal, respectively. Let  $5 \times 5$  minimal evaluation matrices  $\mathbf{A}^{i,j} = X_{i,j}^{0,0} \cdot \mathbf{Z}$ , and  $5 \times 5$  fundamental matrices  $\mathbf{B}^{i,j} = \mathbf{P}_5^{-i} \mathbf{A}^{i,j} \mathbf{Q}_5^{-j}$ , where  $\mathbf{P}_5$  and  $\mathbf{Q}_5$  are defined by Eq.(2) with  $M = N = 5$ ,  $i = 0, 1, 2$ , and  $j = 0, 1, 2$ .  $\mathbf{A}^{i,j}$ 's and  $\mathbf{B}^{i,j}$ 's are shown in Fig.1<sup>1</sup>.

### 2.1 Correlation of $\mathbf{X}^{0,0}$ and $\mathbf{Z}$

It is clear that  $\mathbf{X}^{0,0} \diamond \mathbf{Z}(0,0) = \langle (1, 2, 3, 4, 5, 6, 7, 8, 9), (a, b, c, f, g, h, k, l, m) \rangle$ . According to the construction of  $\mathbf{A}^{i,j}$ 's and  $\mathbf{B}^{i,j}$ 's,  $X_{i,j}^{0,0} \cdot Z_{i,j} = B_{0,0}^{i,j}$ ,  $i = 0, 1, 2$  and  $j = 0, 1, 2$ .  $X_{i,j}^{0,0} \cdot Z_{i,j}$ 's are marked by the blue blocks in Fig.1(b). Therefore,

$$\mathbf{X}^{0,0} \diamond \mathbf{Z}(0,0) = \sum_{i=0}^2 \sum_{j=0}^2 B_{0,0}^{i,j}.$$

---

<sup>1</sup>All the numbers of equations and figures refer to the equations and figures of this supplementary material.



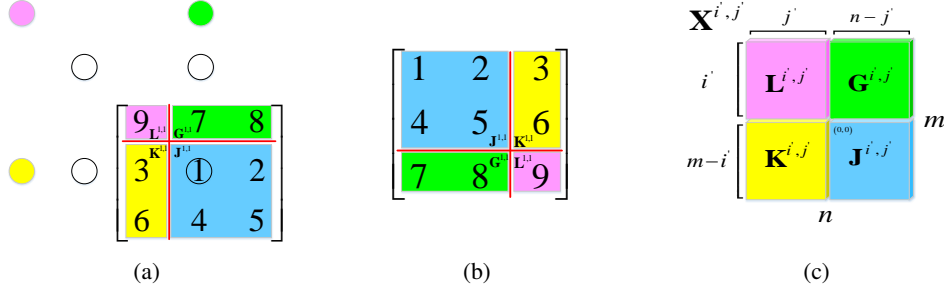

Figure 2: (a) Based on the position of  $\mathbf{X}_{0,0}^{0,0}$ ,  $\mathbf{X}^{1,1}$  is divided into four parts,  $\mathbf{L}^{1,1} = (9)$ ,  $\mathbf{G}^{1,1} = (7, 8)$ ,  $\mathbf{K}^{1,1} = (3, 6)$ , and  $\mathbf{J}^{1,1} = (1, 2, 4, 5)$ . There are pink, green, yellow, and blue blocks. Each color block indicates that the items of correlation  $\mathbf{X}^{1,1} \diamond \mathbf{Z}$ , which contain the elements covered by that color block as their factors, locate the identical position of different fundamental matrices  $\mathbf{B}^{i,j}$ 's. See Sec.2.2 for details. (b) The positions of  $\mathbf{L}^{1,1}$ ,  $\mathbf{G}^{1,1}$ ,  $\mathbf{K}^{1,1}$ , and  $\mathbf{J}^{1,1}$  in  $\mathbf{X}^{0,0}$ . (c) The division of a general circulant correlation filter  $\mathbf{X}^{i',j'}$  into four parts,  $\mathbf{L}^{i',j'}$ ,  $\mathbf{G}^{i',j'}$ ,  $\mathbf{K}^{i',j'}$ , and  $\mathbf{J}^{i',j'}$  by the position of  $\mathbf{X}_{0,0}^{0,0}$ .

Similarly,  $\mathbf{X}^{0,0} \diamond \mathbf{Z}(i'', j'') = \langle (1, 2, 3, 4, 5, 6, 7, 8, 9), \mathbf{z}_{j;i'',j''}^{0,0} \rangle$ , where

$$\mathbf{z}_{j;i'',j''}^{0,0} \triangleq (Z_{i'',j''}, Z_{i'',j''+1}, Z_{i'',j''+2}, \\ Z_{i''+1,j''}, Z_{i''+1,j''+1}, Z_{i''+1,j''+2}, \\ Z_{i''+2,j''}, Z_{i''+2,j''+1}, Z_{i''+2,j''+2}),$$

$i'' = 0, 1, 2$  and  $j'' = 0, 1, 2$ , and  $X_{i,j}^{0,0} \cdot Z_{i''+i,j''+j} = B_{i'',j''}^{i,j}$ . Therefore,

$$\mathbf{X}^{0,0} \diamond \mathbf{Z}(i'', j'') = \sum_{i=0}^2 \sum_{j=0}^2 B_{i'',j''}^{i,j},$$

or set  $\mathbf{C}^{0,0} = \sum_{i=0}^2 \sum_{j=0}^2 \mathbf{B}^{i,j}$ , and then

$$\mathbf{X}^{0,0} \diamond \mathbf{Z} = \mathbf{C}^{0,0}((0, 0), (2, 2)).$$

## 2.2 Correlation of $\mathbf{X}^{1,1}$ and $\mathbf{Z}$

In general, as shown in Fig.2(c), any circulant correlation filter  $\mathbf{X}^{i',j'}$  generated with Eq.(1) can always be divided into four parts,  $\mathbf{L}^{i',j'}$ ,  $\mathbf{G}^{i',j'}$ ,  $\mathbf{K}^{i',j'}$ , and  $\mathbf{J}^{i',j'}$  by the position of  $\mathbf{X}_{0,0}^{0,0}$ . Note that  $\mathbf{L}^{i',j'}$  and  $\mathbf{G}^{i',j'}$  or  $\mathbf{L}^{i',j'}$  and  $\mathbf{K}^{i',j'}$  will not exist if  $i' = 0$  or  $j' = 0$ . Further,  $\mathbf{X}^{i',j'} \diamond \mathbf{Z}$  can be achieved through evaluating four sub-correlations,  $d_L^{i',j'}$ ,  $d_G^{i',j'}$ ,  $d_K^{i',j'}$ , and  $d_J^{i',j'}$ , as expressed in Eq.(3). In the following, we will explain how CCIM works with  $\mathbf{X}^{1,1} \diamond \mathbf{Z}$ .

$\mathbf{X}^{1,1}$ , which is shown in Fig.2(a), is generated with  $i' = j' = 1$ , and  $m = n = 3$ .  $\mathbf{X}^{1,1}$  can be divided into four parts,  $\mathbf{L}^{1,1}$ ,  $\mathbf{G}^{1,1}$ ,  $\mathbf{K}^{1,1}$ , and  $\mathbf{J}^{1,1}$ . Fig.2(b) presents their original positions in  $\mathbf{X}^{0,0}$ . According to Eq.(3), we have

$$\mathbf{X}^{1,1} \diamond \mathbf{Z}(i'', j'') = \langle \mathbf{L}^{1,1}, \mathbf{z}_{L;i'',j''}^{1,1} \rangle + \langle \mathbf{G}^{1,1}, \mathbf{z}_{G;i'',j''}^{1,1} \rangle + \\ \langle \mathbf{K}^{1,1}, \mathbf{z}_{K;i'',j''}^{1,1} \rangle + \langle \mathbf{J}^{1,1}, \mathbf{z}_{J;i'',j''}^{1,1} \rangle,$$

where  $\mathbf{L}^{1,1} = (9)$ ,  $\mathbf{z}_{L;i'',j''}^{1,1} = (Z_{i'',j''})$ ,  $\mathbf{G}^{1,1} = (7, 8)$ ,  $\mathbf{z}_{G;i'',j''}^{1,1} = (Z_{i'',j''+1}, Z_{i'',j''+2})$ ,  $\mathbf{K}^{1,1} = (3, 6)$ ,  $\mathbf{z}_{K;i'',j''}^{1,1} = (Z_{i''+1,j''}, Z_{i''+2,j''})$ ,  $\mathbf{J}^{1,1} = (1, 2, 4, 5)$ , and  $\mathbf{z}_{J;i'',j''}^{1,1} = (Z_{i''+1,j''+1}, Z_{i''+1,j''+2}, Z_{i''+2,j''+1}, Z_{i''+2,j''+2})$ , and

$$\mathbf{X}^{1,1} \diamond \mathbf{Z} = \mathbf{L}^{1,1} \diamond \mathbf{Z}_L^{1,1} + \mathbf{G}^{1,1} \diamond \mathbf{Z}_G^{1,1} + \mathbf{K}^{1,1} \diamond \mathbf{Z}_K^{1,1} + \mathbf{J}^{1,1} \diamond \mathbf{Z}_J^{1,1},$$

where  $\mathbf{Z}_L^{1,1} = \mathbf{Z}((0, 0), (2, 2))$ ,  $\mathbf{Z}_G^{1,1} = \mathbf{Z}((0, 1), (2, 4))$ ,  $\mathbf{Z}_K^{1,1} = \mathbf{Z}((1, 0), (4, 2))$ , and  $\mathbf{Z}_J^{1,1} = \mathbf{Z}((1, 1), (4, 4))$ .

While  $(i'', j'') = (0, 0)$ , we have  $\mathbf{z}_{L;0,0}^{1,1} = (a)$ ,  $\mathbf{z}_{G;0,0}^{1,1} = (b, c)$ ,  $\mathbf{z}_{K;0,0}^{1,1} = (f, k)$ ,  $\mathbf{z}_{J;0,0}^{1,1} = (g, h, l, m)$ , and  $\langle \mathbf{L}^{1,1}, \mathbf{z}_{L;0,0}^{1,1} \rangle = 9a$ . According to Fig.1(c),  $\langle \mathbf{L}^{1,1}, \mathbf{z}_{L;0,0}^{1,1} \rangle = B_{3,3}^{2,2}$  which is marked by the pink block in  $\mathbf{B}^{2,2}$  of Fig.1(c)<sup>2</sup>.

It can be seen from Fig.1(c) that while  $(i'', j'')$  traverses all elements of  $S = \{(i'', j'') | i'' = 0, 1, 2; j'' = 0, 1, 2\}$ ,  $\langle \mathbf{L}^{1,1}, \mathbf{z}_{L;i'',j''}^{1,1} \rangle$  produces nine values,  $9a, 9b, 9c, 9f, 9g, 9h, 9k, 9l$ , and  $9m$ . Suppose the 0<sup>th</sup> and 4<sup>th</sup> rows are adjacent, and the 0<sup>th</sup> and 4<sup>th</sup> columns are adjacent too in  $\mathbf{B}^{i,j,s}$ . Then, the 9 values consist of a sub-matrix of  $\mathbf{B}^{2,2}$ , which is marked by a red bounding box in  $\mathbf{B}^{2,2}$  of Fig.1(c). Set  $\mathbf{S}_L^{1,1} = \mathbf{B}^{2,2}$ . Cyclically shifting the marked sub-matrix to the top left corner of  $\mathbf{S}_L^{1,1}$ , we achieve

$$\mathbf{L}^{1,1} \diamond \mathbf{Z}_L^{1,1} = \mathbf{S}_L^{1,1}((0, 0), (2, 2)).$$

Similarly, while  $(i'', j'') = (0, 0)$ ,  $\langle \mathbf{G}^{1,1}, \mathbf{z}_{G;0,0}^{1,1} \rangle = 7b + 8c = B_{3,1}^{2,0} + B_{3,1}^{2,1}$ ,  $B_{3,1}^{2,0}$  and  $B_{3,1}^{2,1}$  are marked with two green blocks in  $\mathbf{B}^{2,0}$  and  $\mathbf{B}^{2,1}$  of Fig.1(c). While  $(i'', j'')$  traverses all elements of  $S = \{(i'', j'') | i'' = 0, 1, 2; j'' = 0, 1, 2\}$ ,  $\langle \mathbf{G}^{1,1}, \mathbf{z}_{G;i'',j''}^{1,1} \rangle$  produces nine values,  $7b + 8c, 7c + 8d, 7d + 8e, 7g + 8h, 7h + 8i, 7i + 8j, 7l + 8m, 7m + 8n$ , and  $7n + 8o$ . Observe the sub-matrices of  $\mathbf{B}^{2,0}$  and  $\mathbf{B}^{2,1}$  which are marked by two red bounding boxes in  $\mathbf{B}^{2,0}$  and  $\mathbf{B}^{2,1}$  of Fig.1(c). These nine values are just the elements of the summation of the two sub-matrices. Cyclically shifting the marked sub-matrices to the top left corners of  $\mathbf{B}^{2,0}$  and  $\mathbf{B}^{2,1}$ , and setting  $\mathbf{S}_G^{1,1} = \mathbf{B}^{2,0} + \mathbf{B}^{2,1}$ , we achieve

$$\mathbf{G}^{1,1} \diamond \mathbf{Z}_G^{1,1} = \mathbf{S}_G^{1,1}((0, 0), (2, 2)).$$

Similarly, while  $(i'', j'') = (0, 0)$ ,  $\langle \mathbf{K}^{1,1}, \mathbf{z}_{K;0,0}^{1,1} \rangle = 3f + 6k = B_{1,3}^{0,2} + B_{1,3}^{1,2}$ ,  $B_{1,3}^{0,2}$  and  $B_{1,3}^{1,2}$  are marked with two yellow blocks in  $\mathbf{B}^{0,2}$  and  $\mathbf{B}^{1,2}$  of Fig.1(c). While  $(i'', j'')$  traverses all elements of  $S = \{(i'', j'') | i'' = 0, 1, 2; j'' = 0, 1, 2\}$ ,  $\langle \mathbf{K}^{1,1}, \mathbf{z}_{K;i'',j''}^{1,1} \rangle$  produces nine values,  $3f + 6k, 3g + 6l, 3h + 6m, 3k + 6p, 3l + 6q, 3m + 6r, 3p + 6u, 3q + 6w$ , and  $3r + 6x$ . Observe the sub-matrices of  $\mathbf{B}^{0,2}$  and  $\mathbf{B}^{1,2}$  which are marked by two red bounding boxes in  $\mathbf{B}^{0,2}$  and  $\mathbf{B}^{1,2}$  of Fig.1(c). These nine values are just the elements of the summation of the two sub-matrices. Cyclically shifting the marked sub-matrices to the top left corners of  $\mathbf{B}^{0,2}$  and  $\mathbf{B}^{1,2}$ , and setting  $\mathbf{S}_K^{1,1} = \mathbf{B}^{0,2} + \mathbf{B}^{1,2}$ , we achieve

$$\mathbf{K}^{1,1} \diamond \mathbf{Z}_K^{1,1} = \mathbf{S}_K^{1,1}((0, 0), (2, 2)).$$

Similarly, while  $(i'', j'') = (0, 0)$ ,  $\langle \mathbf{J}^{1,1}, \mathbf{z}_{J;0,0}^{1,1} \rangle = 1g + 2h + 4l + 5m = B_{1,1}^{0,0} + B_{1,1}^{0,1} + B_{1,1}^{1,0} + B_{1,1}^{1,1}$ ,  $B_{1,1}^{0,0}$ ,  $B_{1,1}^{0,1}$ ,  $B_{1,1}^{1,0}$ , and  $B_{1,1}^{1,1}$  are marked with four blue blocks in  $\mathbf{B}^{0,0}$ ,  $\mathbf{B}^{0,1}$ ,  $\mathbf{B}^{1,0}$  and  $\mathbf{B}^{1,1}$  of Fig.1(c). While  $(i'', j'')$  traverses all elements of  $S = \{(i'', j'') | i'' = 0, 1, 2; j'' = 0, 1, 2\}$ ,  $\langle \mathbf{J}^{1,1}, \mathbf{z}_{J;i'',j''}^{1,1} \rangle$  produces nine values,  $1g + 2h + 4l + 5m, 1h + 2i + 4m + 5n, 1i + 2j + 4n + 5o, 1l + 2m + 4q + 5r, 1m + 2n + 4r + 5s, 1n + 2o + 4s + 5t, 1q + 2r + 4w + 5x, 1r + 2s + 4x + 5y$ , and  $1s + 2t + 4y + 5z$ . Observe the sub-matrices of  $\mathbf{B}^{0,0}$ ,  $\mathbf{B}^{0,1}$ ,  $\mathbf{B}^{1,0}$  and  $\mathbf{B}^{1,1}$  which are marked by four red bounding boxes in  $\mathbf{B}^{0,0}$ ,  $\mathbf{B}^{0,1}$ ,  $\mathbf{B}^{1,0}$  and  $\mathbf{B}^{1,1}$  of Fig.1(c). These nine values are just the elements of the summation of the four sub-matrices. Cyclically shifting the marked sub-matrices to the top left corners of  $\mathbf{B}^{0,0}$ ,  $\mathbf{B}^{0,1}$ ,  $\mathbf{B}^{1,0}$  and  $\mathbf{B}^{1,1}$ , and setting  $\mathbf{S}_J^{1,1} = \mathbf{B}^{0,0} + \mathbf{B}^{0,1} + \mathbf{B}^{1,0} + \mathbf{B}^{1,1}$ , we achieve

$$\mathbf{J}^{1,1} \diamond \mathbf{Z}_J^{1,1} = \mathbf{S}_J^{1,1}((0, 0), (2, 2)).$$

Finally, set  $\mathbf{C}^{1,1} = \sum_{W \in \{L, G, K, J\}} \mathbf{S}_W^{1,1}$ , then,

$$\mathbf{X}^{1,1} \diamond \mathbf{Z} = \mathbf{C}^{1,1}((0, 0), (2, 2)).$$

<sup>2</sup>In fact, according to the example in Sec.2.1 and Fig.2(b), the item with 9 as its factor should be shifted to the position marked with the pink circle in Fig.2(a). Therefore,  $\langle \mathbf{L}^{1,1}, \mathbf{z}_{L;0,0}^{1,1} \rangle = 9a$  should be shifted to the position marked with the pink circle. Then,  $9a$  is shifted to  $(3, 3)$  of  $\mathbf{B}^{2,2}$  according to the construction of  $\mathbf{B}^{2,2}$  through the cyclic-shift of  $\mathbf{A}^{2,2}$ . Similarly, the items produced by  $\langle \mathbf{G}^{1,1}, \mathbf{z}_{G;0,0}^{1,1} \rangle$  and  $\langle \mathbf{K}^{1,1}, \mathbf{z}_{K;0,0}^{1,1} \rangle$  should be shifted to the positions marked with green and yellow circles, respectively. According to the same reason, these items are shifted to the  $(3, 1)$ 's of  $\mathbf{B}^{2,0}$  and  $\mathbf{B}^{2,1}$ , and the  $(1, 3)$ 's of  $\mathbf{B}^{0,2}$  and  $\mathbf{B}^{1,2}$ , respectively. Finally, the four items generated by  $\langle \mathbf{J}^{1,1}, \mathbf{z}_{J;0,0}^{1,1} \rangle$  are shifted to the position marked by the blue circle, i.e.,  $(1, 1)$ 's of  $\mathbf{B}^{0,0}$ ,  $\mathbf{B}^{0,1}$ ,  $\mathbf{B}^{1,0}$  and  $\mathbf{B}^{1,1}$ .

### 2.3 Design Integral Matrix to Accelerate Correlation

According to the beginning of this section,  $X_{i,j}^{0,0}$  is the common factor of all elements of  $\mathbf{B}^{i,j}$ . Replacing  $X_{i,j}^{0,0}$  by  $\mathbf{B}^{i,j}$  in  $\mathbf{X}^{0,0}$ , we achieve

$$\mathbf{T} = \begin{bmatrix} \mathbf{B}^{0,0} & \mathbf{B}^{0,1} & \mathbf{B}^{0,2} \\ \mathbf{B}^{1,0} & \mathbf{B}^{1,1} & \mathbf{B}^{1,2} \\ \mathbf{B}^{2,0} & \mathbf{B}^{2,1} & \mathbf{B}^{2,2} \end{bmatrix}.$$

Based on the examples given in Secs.2.1 and 2.2, it is necessary to evaluate  $\sum_{i=0}^2 \sum_{j=0}^2 \mathbf{B}^{i,j}$  to achieve  $\mathbf{X}^{0,0} \diamond \mathbf{Z}$ , and to evaluate  $\mathbf{B}^{2,2}$ ,  $\mathbf{B}^{2,0} + \mathbf{B}^{2,1}$ ,  $\mathbf{B}^{0,2} + \mathbf{B}^{1,2}$ , and  $\mathbf{B}^{0,0} + \mathbf{B}^{0,1} + \mathbf{B}^{1,0} + \mathbf{B}^{1,1}$  to obtain  $\mathbf{X}^{1,1} \diamond \mathbf{Z}$ . In order to eliminate unnecessary additions, the three summations of matrices, which are necessary for evaluating  $\mathbf{X}^{1,1} \diamond \mathbf{Z}$ , should be reused to evaluate  $\mathbf{X}^{0,0} \diamond \mathbf{Z}$ . Notice that each above summation of  $\mathbf{B}^{i,j}$ 's is involved with the summation of the elements of  $\mathbf{T}$ 's sub-matrices. Constructing the integral matrix  $\mathbf{M}_\mathbf{I}$  with CCIM, we have

$$\mathbf{M}_\mathbf{I} = \begin{bmatrix} \mathbf{M}_{0,0} & \mathbf{M}_{0,1} & \mathbf{M}_{0,2} \\ \mathbf{M}_{1,0} & \mathbf{M}_{1,1} & \mathbf{M}_{1,2} \\ \mathbf{M}_{2,0} & \mathbf{M}_{2,1} & \mathbf{M}_{2,2} \end{bmatrix},$$

where  $\mathbf{M}_{s,t} = \sum_{0 \leq i \leq s, 0 \leq j \leq t} \mathbf{B}^{i,j}$ . Then,  $\mathbf{M}_{2,2} = \sum_{i=0}^2 \sum_{j=0}^2 \mathbf{B}^{i,j}$ ,  $\mathbf{M}_{2,2} - \mathbf{M}_{1,2} - \mathbf{M}_{2,1} + \mathbf{M}_{1,1} = \mathbf{B}^{2,2}$ ,  $\mathbf{M}_{2,1} - \mathbf{M}_{1,1} = \mathbf{B}^{2,0} + \mathbf{B}^{2,1}$ ,  $\mathbf{M}_{1,2} - \mathbf{M}_{1,1} = \mathbf{B}^{0,2} + \mathbf{B}^{1,2}$ , and  $\mathbf{M}_{1,1} = \mathbf{B}^{0,0} + \mathbf{B}^{0,1} + \mathbf{B}^{1,0} + \mathbf{B}^{1,1}$ . It is seen that the five summations of  $\mathbf{B}^{i,j}$ 's are achieved within constant duration by means of  $\mathbf{M}_\mathbf{I}$ . This way, the unnecessary additions of  $\mathbf{B}^{i,j}$ 's are eliminated.

In general, because  $\mathbf{W}^{i',j'}$  is a sub-matrix of  $\mathbf{X}^{0,0}$ , where  $\mathbf{W} = \mathbf{L}, \mathbf{G}, \mathbf{K}, \mathbf{J}$ , the  $\mathbf{B}^{i,j}$ 's with the elements of  $\mathbf{W}$  as their common factors also constitute a  $\mathbf{T}$ 's sub-matrix. While evaluating  $d_W^{i',j'}$ , where  $W \in \{L, G, K, J\}$ , similar to the examples in Secs.2.1 and 2.2, it is necessary to evaluate the summation of all elements of the  $\mathbf{T}$ 's sub-matrix. For a given  $\mathbf{X}^{0,0}$ , while  $(i', j')$  traverses all possible pairs, i.e.,  $\mathbf{X}^{i',j'}$  traverses all possible circulant correlation filters, the brute force evaluation of the summations will arise a great deal of unnecessary computation, decreasing the efficiency of correlations greatly especially when the size of base correlation filter is large. Therefore, it is a natural choice to construct the integral matrix, as described in CCIM, to calculate such summations without unnecessary additions.

### 3 Correctness of Algorithm 2 (CCIM)

Suppose  $\mathbf{X}^{0,0} \in \mathbb{R}^{m \times n \times D}$  is the  $m \times n \times D$  base correlation filter with  $X_{i,j,d}^{0,0}$  as its elements,  $(i, j)$  is the spatial coordinate,  $d$  is the channel, circulant correlation filters

$$\mathbf{X}^{i',j'} = \mathbf{P}_m^{i'} \mathbf{X}^{0,0} \mathbf{Q}_n^{j'}, \quad i' = 0, \dots, m-1, \quad j' = 0, \dots, n-1, \quad (1)$$

where  $\mathbf{P}_{l_1}, l_1 \in \{m, M\}$ , and  $\mathbf{Q}_{l_2}, l_2 \in \{n, N\}$ , are the permutation matrices of  $l_1 \times l_1$  and  $l_2 \times l_2$ , respectively [3],

$$\mathbf{P}_{l_1} = \begin{bmatrix} \mathbf{0}_{l_1-1}^\top & \mathbf{1} \\ \mathbf{I}_{l_1-1} & \mathbf{0}_{l_1-1} \end{bmatrix}, \quad \mathbf{Q}_{l_2} = \begin{bmatrix} \mathbf{0}_{l_2-1} & \mathbf{I}_{l_2-1} \\ \mathbf{1} & \mathbf{0}_{l_2-1}^\top \end{bmatrix}, \quad (2)$$

$\mathbf{P}_{l_1}^\rho$  and  $\mathbf{Q}_{l_2}^\rho$  are the  $\rho^{\text{th}}$  power of  $\mathbf{P}_{l_1}$  and  $\mathbf{Q}_{l_2}$ , respectively,  $\mathbf{0}_{l-1}$  is  $(l-1) \times 1$  vector of all zeros,  $\mathbf{I}_{l-1}$  is  $(l-1) \times (l-1)$  identity matrix,  $l \in \{l_1, l_2\}$ . Note that the matrix operation works only on the spatial coordinate in Eq.(1).  $\mathbf{Z} \in \mathbb{R}^{M \times N \times D}$  is the  $M \times N \times D$  signal matrix with  $Z_{i'',j'',d}$  as its elements.  $\mathbf{Z}_d \in \mathbb{R}^{M \times N}$  is its  $d^{\text{th}}$  channel matrix.

Let  $M \times N$  minimal evaluation matrix  $\mathbf{A}^{i,j} = \sum_{d=0}^{D-1} X_{i,j,d}^{0,0} \cdot \mathbf{Z}_d$ , where  $i = 0, \dots, m-1, j = 0, \dots, n-1$ , and  $M \times N$  fundamental matrix  $\mathbf{B}^{i,j} = \mathbf{P}_M^{-i} \mathbf{A}^{i,j} \mathbf{Q}_N^{-j}$ . Note that  $\mathbf{B}^{i,j}$ 's are generated through cyclic-shifts of  $\mathbf{A}^{i,j}$ . Then,  $X_{i,j}^{0,0}$  only appears in  $\mathbf{A}^{i,j}$  and  $\mathbf{B}^{i,j}$  as a common factor of their elements. The sets of whole  $\mathbf{A}^{i,j}$ 's and  $\mathbf{B}^{i,j}$ 's are denoted as  $\mathfrak{A}$  and  $\mathfrak{B}$ , respectively.

In this appendix, we will prove that CCIM will produce  $\mathbf{X}^{i',j'} \diamond \mathbf{Z}$  correctly. To simplify the mathematical expression, we only present our proof in the case of  $D = 1$ . It is straightforward to extend the proof to the general case of  $D > 1$ .

In general, as shown in Fig.2(c), given  $i'$  and  $j'$ ,  $\mathbf{X}^{i',j'}$  can always be divided into four parts,  $\mathbf{L}^{i',j'}$ ,  $\mathbf{G}^{i',j'}$ ,  $\mathbf{K}^{i',j'}$ , and  $\mathbf{J}^{i',j'}$  by the position of  $X_{0,0}^{0,0}$ .  $\mathbf{L}^{i',j'}$ ,  $\mathbf{G}^{i',j'}$ ,  $\mathbf{K}^{i',j'}$ , and  $\mathbf{J}^{i',j'}$  are  $i' \times j'$ ,  $i' \times (n - j')$ ,  $(m - i') \times j'$ , and  $(m - i') \times (n - j')$ , respectively, and their top left elements are  $L_{0,0}^{i',j'} = X_{m-i',n-j'}^{0,0}$ ,  $G_{0,0}^{i',j'} = X_{m-i',0}^{0,0}$ ,  $K_{0,0}^{i',j'} = X_{0,n-j'}^{0,0}$ , and  $J_{0,0}^{i',j'} = X_{0,0}^{0,0}$ , respectively. Note that  $\mathbf{L}^{i',j'}$  and  $\mathbf{G}^{i',j'}$  or  $\mathbf{L}^{i',j'}$  and  $\mathbf{K}^{i',j'}$  will not exist if  $i' = 0$  or  $j' = 0$ .

Let

$$\begin{aligned} \mathbf{X}^{i',j'} \diamond \mathbf{Z}(i'', j'') &= \sum_{s=0}^{m-1} \sum_{t=0}^{n-1} X_{s,t}^{i',j'} \cdot Z_{i''+s, j''+t} \\ &= d_L^{i',j'}(i'', j'') + d_G^{i',j'}(i'', j'') + d_K^{i',j'}(i'', j'') + d_J^{i',j'}(i'', j''), \end{aligned} \quad (3)$$

where

$$\begin{aligned} d_L^{i',j'}(i'', j'') &= \sum_{s=0}^{i'-1} \sum_{t=0}^{j'-1} X_{s,t}^{i',j'} \cdot Z_{i''+s, j''+t} \\ &= \langle \mathbf{L}^{i',j'}, \mathbf{Z}((i'', j''), (i'' + i' - 1, j'' + j' - 1)) \rangle, \\ d_G^{i',j'}(i'', j'') &= \sum_{s=0}^{i'-1} \sum_{t=j'}^{n-1} X_{s,t}^{i',j'} \cdot Z_{i''+s, j''+t} \\ &= \langle \mathbf{G}^{i',j'}, \mathbf{Z}((i'', j'' + j'), (i'' + i' - 1, j'' + n - 1)) \rangle, \\ d_K^{i',j'}(i'', j'') &= \sum_{s=i'}^{m-1} \sum_{t=0}^{j'-1} X_{s,t}^{i',j'} \cdot Z_{i''+s, j''+t} \\ &= \langle \mathbf{K}^{i',j'}, \mathbf{Z}((i'' + i', j''), (i'' + m - 1, j'' + j' - 1)) \rangle, \\ d_J^{i',j'}(i'', j'') &= \sum_{s=i'}^{m-1} \sum_{t=j'}^{n-1} X_{s,t}^{i',j'} \cdot Z_{i''+s, j''+t} \\ &= \langle \mathbf{J}^{i',j'}, \mathbf{Z}((i'' + i', j'' + j'), (i'' + m - 1, j'' + n - 1)) \rangle, \end{aligned}$$

$i'' = 0, \dots, M - m$ , and  $j'' = 0, \dots, N - n$ .

### 3.1 Evaluation of $d_L^{i',j'}(i'', j'')$

While evaluating  $d_L^{i',j'}(i'', j'')$ ,  $L_{0,0}^{i',j'}$  and  $Z_{i'', j''}$  multiply. According to the construction of  $\mathfrak{A}$  and  $\mathfrak{B}$ , we have

$$L_{0,0}^{i',j'} \cdot Z_{i'', j''} = A_{i'', j''}^{m-i', n-j'}.$$

Because

$$\mathbf{B}^{m-i', n-j'} = \mathbf{P}_M^{-(m-i')} \mathbf{A}^{m-i', n-j'} \mathbf{Q}_N^{-(n-j')},$$

therefore

$$L_{0,0}^{i',j'} \cdot Z_{i'', j''} = B_{(i''-(m-i')) \bmod M, (j''-(n-j')) \bmod N}^{m-i', n-j'}.$$

On the other hand,  $L_{p,q}^{i',j'} = X_{m-i'+p, n-j'+q}^{0,0}$ , where  $p = 0, \dots, i' - 1$  and  $q = 0, \dots, j' - 1$ . It only appears in  $\mathbf{B}^{m-i'+p, n-j'+q}$ , and

$$L_{p,q}^{i',j'} \cdot Z_{i''+p, j''+q} = A_{i''+p, j''+q}^{m-i'+p, n-j'+q}.$$

We also have

$$\begin{aligned} \mathbf{B}^{m-i'+p, n-j'+q} &= \mathbf{P}_M^{-(m-i'+p)} \mathbf{A}^{m-i'+p, n-j'+q} \mathbf{Q}_N^{-(n-j'+q)} \\ &= \mathbf{P}_M^{-(m-i')} \mathbf{P}_M^{-p} \mathbf{A}^{m-i'+p, n-j'+q} \mathbf{Q}_N^{-q} \mathbf{Q}_N^{-(n-j')}. \end{aligned}$$

Let

$$\mathbf{A}^{(L)} = \mathbf{P}_M^{-p} \mathbf{A}^{m-i'+p, n-j'+q} \mathbf{Q}_N^{-q}.$$

Then,  $A_{i'', j''}^{(L)} = A_{i''+p, j''+q}^{m-i'+p, n-j'+q}$ . That is,  $L_{p, q}^{i', j'} \cdot Z_{i''+p, j''+q} = A_{i'', j''}^{(L)}$ . Because

$$\mathbf{B}^{m-i'+p, n-j'+q} = \mathbf{P}_M^{-(m-i')} \mathbf{A}^{(L)} \mathbf{Q}_N^{-(n-j')},$$

therefore

$$L_{p, q}^{i', j'} \cdot Z_{i''+p, j''+q} = B_{(i''-(m-i')) \bmod M, (j''-(n-j')) \bmod N}^{m-i'+p, n-j'+q}.$$

That is,  $L_{0,0}^{i', j'}$  and  $L_{p, q}^{i', j'}$  possess the same subscripts, although they belong to different fundamental matrices.

It is seen from Fig.2(c) that the top left and bottom right elements of  $\mathbf{L}^{i', j'}$  are  $(X_{m-i', n-j'}^{0,0}, X_{m-1, n-1}^{0,0})$ . Let  $\mathbf{S}^{L, i', j'} = \sum_{i=m-i'}^{m-1} \sum_{j=n-j'}^{n-1} \mathbf{B}^{i, j}$ . According to the construction of integral matrix,  $\mathbf{S}^{L, i', j'}$  can be evaluated within constant time as

$$\mathbf{S}^{L, i', j'} = \mathbf{M}_{m-1, n-1} - \mathbf{M}_{m-1, n-j'-1} - \mathbf{M}_{m-i'-1, n-1} + \mathbf{M}_{m-i'-1, n-j'-1}.$$

Then, we have

$$d_L^{i', j'}(i'', j'') = S_{(i''-(m-i')) \bmod M, (j''-(n-j')) \bmod N}^{L, i', j'}.$$

### 3.2 Evaluation of $d_G^{i', j'}(i'', j'')$

While evaluating  $d_G^{i', j'}(i'', j'')$ ,  $G_{0,0}^{i', j'}$  and  $Z_{i'', j''+j'}$  multiply. According to the construction of  $\mathfrak{A}$  and  $\mathfrak{B}$ , we have

$$G_{0,0}^{i', j'} \cdot Z_{i'', j''+j'} = A_{i'', j''+j'}^{m-i', 0}.$$

Because

$$\mathbf{B}^{m-i', 0} = \mathbf{P}_M^{-(m-i')} \mathbf{A}^{m-i', 0},$$

therefore

$$G_{0,0}^{i', j'} \cdot Z_{i'', j''+j'} = B_{(i''-(m-i')) \bmod M, j''+j'}^{m-i', 0}.$$

On the other hand,  $G_{p, q}^{i', j'} = X_{m-i'+p, q}^{0,0}$ , where  $p = 0, \dots, i' - 1$  and  $q = 0, \dots, n - j' - 1$ . It only appears in  $\mathbf{B}^{m-i'+p, q}$ , and

$$G_{p, q}^{i', j'} \cdot Z_{i''+p, j''+j'+q} = A_{i''+p, j''+j'+q}^{m-i'+p, q}.$$

We also have

$$\begin{aligned} \mathbf{B}^{m-i'+p, q} &= \mathbf{P}_M^{-(m-i'+p)} \mathbf{A}^{m-i'+p, q} \mathbf{Q}_N^{-q} \\ &= \mathbf{P}_M^{-(m-i')} \mathbf{P}_M^{-p} \mathbf{A}^{m-i'+p, q} \mathbf{Q}_N^{-q}. \end{aligned}$$

Let

$$\mathbf{A}^{(G)} = \mathbf{P}_M^{-p} \mathbf{A}^{m-i'+p, q} \mathbf{Q}_N^{-q}.$$

Then,  $A_{i'', j''+j'}^{(G)} = A_{i''+p, j''+j'+q}^{m-i'+p, q}$ . That is,  $G_{p, q}^{i', j'} \cdot Z_{i''+p, j''+j'+q} = A_{i'', j''+j'}^{(G)}$ . Because

$$\mathbf{B}^{m-i'+p, q} = \mathbf{P}_M^{-(m-i')} \mathbf{A}^{(G)},$$

therefore

$$G_{p, q}^{i', j'} \cdot Z_{i''+p, j''+j'+q} = B_{(i''-(m-i')) \bmod M, j''+j'+q}^{m-i'+p, q}.$$

That is,  $G_{0,0}^{i', j'}$  and  $L_{p, q}^{i', j'}$  possess the same subscripts, although they belong to different fundamental matrices.

It is seen from Fig.2(c) that the top left and bottom right elements of  $\mathbf{G}^{i', j'}$  are  $(X_{m-i', 0}^{0,0}, X_{m-1, n-j'-1}^{0,0})$ . Let  $\mathbf{S}^{G, i', j'} = \sum_{i=m-i'}^{m-1} \sum_{j=0}^{n-j'-1} \mathbf{B}^{i, j}$ . According to the construction of integral matrix,  $\mathbf{S}^{G, i', j'}$  can be evaluated within constant time as

$$\mathbf{S}^{G, i', j'} = \mathbf{M}_{m-1, n-j'-1} - \mathbf{M}_{m-i'-1, n-j'-1}.$$

Then, we have

$$d_G^{i', j'}(i'', j'') = S_{(i''-(m-i')) \bmod M, j''+j'}^{G, i', j'}.$$

### 3.3 Evaluation of $d_K^{i',j'}(i'',j'')$

While evaluating  $d_K^{i',j'}(i'',j'')$ ,  $K_{0,0}^{i',j'}$  and  $Z_{i''+i',j''}$  multiply. According to the construction of  $\mathfrak{A}$  and  $\mathfrak{B}$ , we have

$$K_{0,0}^{i',j'} \cdot Z_{i''+i',j''} = A_{i''+i',j''}^{0,n-j'}.$$

Because

$$\mathbf{B}^{0,n-j'} = \mathbf{A}^{0,n-j'} \mathbf{Q}_N^{-(n-j')},$$

therefore

$$K_{0,0}^{i',j'} \cdot Z_{i''+i',j''} = B_{i''+i',(j''-(n-j')) \bmod N}^{0,n-j'}.$$

On the other hand,  $K_{p,q}^{i',j'} = X_{p,n-j'+q}^{0,0}$ , where  $p = 0, \dots, m-i'-1$  and  $q = 0, \dots, j'-1$ . It only appears in  $\mathbf{B}^{p,n-j'+q}$ , and

$$K_{p,q}^{i',j'} \cdot Z_{i''+i'+p,j''+q} = A_{i''+i'+p,j''+q}^{p,n-j'+q}.$$

We also have

$$\begin{aligned} \mathbf{B}^{p,n-j'+q} &= \mathbf{P}_M^{-p} \mathbf{A}^{p,n-j'+q} \mathbf{Q}_N^{-(n-j'+q)} \\ &= \mathbf{P}_M^{-p} \mathbf{A}^{p,n-j'+q} \mathbf{Q}_N^{-q} \mathbf{Q}_N^{-(n-j')}. \end{aligned}$$

Let

$$\mathbf{A}^{(K)} = \mathbf{P}_M^{-p} \mathbf{A}^{p,n-j'+q} \mathbf{Q}_N^{-q}.$$

Then,  $A_{i''+i',j''}^{(K)} = A_{i''+i'+p,j''+q}^{p,n-j'+q}$ . That is,  $K_{p,q}^{i',j'} \cdot Z_{i''+i'+p,j''+q} = A_{i''+i',j''}^{(K)}$ . Because

$$\mathbf{B}^{p,n-j'+q} = \mathbf{A}^{(K)} \mathbf{Q}_N^{-(n-j')},$$

therefore

$$K_{p,q}^{i',j'} \cdot Z_{i''+i'+p,j''+q} = B_{i''+i',(j''-(n-j')) \bmod N}^{p,n-j'+q}.$$

That is,  $K_{0,0}^{i',j'} \cdot Z_{i''+i',j''}$  and  $K_{p,q}^{i',j'} \cdot Z_{i''+i'+p,j''+q}$  possess the same subscripts, although they belong to different fundamental matrices.

It is seen from Fig.2(c) that the top left and bottom right elements of  $\mathbf{K}^{i',j'}$  are  $(X_{0,n-j'}^{0,0}, X_{m-i'-1,n-1}^{0,0})$ . Let  $\mathbf{S}^{K,i',j'} = \sum_{i=0}^{m-i'-1} \sum_{j=n-j'}^{n-1} \mathbf{B}^{i,j}$ . According to the construction of integral matrix,  $\mathbf{S}^{K,i',j'}$  can be evaluated within constant time as

$$\mathbf{S}^{K,i',j'} = \mathbf{M}_{m-i'-1,n-1} - \mathbf{M}_{m-i'-1,n-j'-1}.$$

Then, we have

$$d_K^{i',j'}(i'',j'') = S_{i''+i',(j''-(n-j')) \bmod N}^{K,i',j'}.$$

### 3.4 Evaluation of $d_J^{i',j'}(i'',j'')$

While evaluating  $d_J^{i',j'}(i'',j'')$ ,  $J_{0,0}^{i',j'}$  and  $Z_{i''+i',j''+j'}$  multiply. According to the construction of  $\mathfrak{A}$  and  $\mathfrak{B}$ , we have  $J_{0,0}^{i',j'} \cdot Z_{i''+i',j''+j'} = A_{i''+i',j''+j'}^{0,0}$ . And  $\mathbf{B}^{0,0} = \mathbf{A}^{0,0}$ . Therefore,  $J_{0,0}^{i',j'} \cdot Z_{i''+i',j''+j'} = B_{i''+i',j''+j'}^{0,0}$ .

On the other hand,  $J_{p,q}^{i',j'} = X_{p,q}^{0,0}$ , where  $p = 0, \dots, m-i'-1$  and  $q = 0, \dots, n-j'-1$ . It only appears in  $\mathbf{B}^{p,q}$ , and

$$J_{p,q}^{i',j'} \cdot Z_{i''+i'+p,j''+j'+q} = A_{i''+i'+p,j''+j'+q}^{p,q}.$$

We also have  $\mathbf{B}^{p,q} = \mathbf{P}_M^{-p} \mathbf{A}^{p,q} \mathbf{Q}_N^{-q}$ . Then,  $B_{i''+i',j''+j'}^{p,q} = A_{i''+i'+p,j''+j'+q}^{p,q}$ . Therefore

$$J_{p,q}^{i',j'} \cdot Z_{i''+i'+p,j''+j'+q} = B_{i''+i',j''+j'}^{p,q}.$$

That is,  $J_{0,0}^{i',j'} \cdot Z_{i''+i',j''+j'}$  and  $J_{p,q}^{i',j'} \cdot Z_{i''+i'+p,j''+j'+q}$  possess the same subscripts, although they belong to different fundamental matrices.

It is seen from Fig.2(c) that the top left and bottom right elements of  $\mathbf{J}^{i',j'}$  are  $(X_{0,0}^{0,0}, X_{m-i'-1,n-j'-1}^{0,0})$ . Let  $\mathbf{S}^{J,i',j'} = \sum_{i=0}^{m-i'-1} \sum_{j=0}^{n-j'-1} \mathbf{B}^{i,j}$ . According to the construction of integral matrix,  $\mathbf{S}^{J,i',j'}$  can be evaluated within constant time as

$$\mathbf{S}^{J,i',j'} = \mathbf{M}_{m-i'-1,n-j'-1}.$$

Then, we have

$$d_J^{i',j'}(i'',j'') = S_{i''+i',j''+j'}^{J,i',j'}.$$

### 3.5 Correlation of $\mathbf{X}^{i',j'}$ and $\mathbf{Z}$

According to the proofs in Secs.3.1, 3.2, 3.3, and 3.4, we can get the  $d_L^{i',j'}(i'',j'')$ 's,  $d_G^{i',j'}(i'',j'')$ 's,  $d_K^{i',j'}(i'',j'')$ 's, and  $d_J^{i',j'}(i'',j'')$ 's for all  $(i'',j'')$ 's. Therefore,  $\mathbf{S}^{L,i',j'}$ ,  $\mathbf{S}^{G,i',j'}$ ,  $\mathbf{S}^{K,i',j'}$ , and  $\mathbf{S}^{J,i',j'}$  include the correlation results between  $\mathbf{L}^{i',j'}$ ,  $\mathbf{G}^{i',j'}$ ,  $\mathbf{K}^{i',j'}$ ,  $\mathbf{J}^{i',j'}$  and their corresponding parts of  $\mathbf{Z}$ .

Let

$$\begin{aligned} \Delta_r^{(L)}(i'',j'') &= (i'' - (m - i')) \bmod M - i'', \\ \Delta_c^{(L)}(i'',j'') &= (j'' - (n - j')) \bmod N - j'', \\ \Delta_r^{(G)}(i'',j'') &= (i'' - (m - i')) \bmod M - i'', \\ \Delta_c^{(G)}(i'',j'') &= j', \\ \Delta_r^{(K)}(i'',j'') &= i', \\ \Delta_c^{(K)}(i'',j'') &= (j'' - (n - j')) \bmod N - j'', \\ \Delta_r^{(J)}(i'',j'') &= i', \\ \Delta_c^{(J)}(i'',j'') &= j', \end{aligned} \tag{4}$$

and

$$\begin{aligned} \mathbf{S}_L^{i',j'} &= \mathbf{P}_M^{-\Delta_r^{(L)}(i'',j'')} \mathbf{S}_{L,i',j'}^{-\Delta_c^{(L)}(i'',j'')} \mathbf{Q}_N^{-\Delta_c^{(L)}(i'',j'')}, \\ \mathbf{S}_G^{i',j'} &= \mathbf{P}_M^{-\Delta_r^{(G)}(i'',j'')} \mathbf{S}_{G,i',j'}^{-\Delta_c^{(G)}(i'',j'')} \mathbf{Q}_N^{-\Delta_c^{(G)}(i'',j'')}, \\ \mathbf{S}_K^{i',j'} &= \mathbf{P}_M^{-\Delta_r^{(K)}(i'',j'')} \mathbf{S}_{K,i',j'}^{-\Delta_c^{(K)}(i'',j'')} \mathbf{Q}_N^{-\Delta_c^{(K)}(i'',j'')}, \\ \mathbf{S}_J^{i',j'} &= \mathbf{P}_M^{-\Delta_r^{(J)}(i'',j'')} \mathbf{S}_{J,i',j'}^{-\Delta_c^{(J)}(i'',j'')} \mathbf{Q}_N^{-\Delta_c^{(J)}(i'',j'')}. \end{aligned}$$

Then,  $d_L^{i',j'}(i'',j'')$ ,  $d_G^{i',j'}(i'',j'')$ ,  $d_K^{i',j'}(i'',j'')$ , and  $d_J^{i',j'}(i'',j'')$  are shifted to  $S_{L;i'',j''}^{i',j'}$ ,  $S_{G;i'',j''}^{i',j'}$ ,  $S_{K;i'',j''}^{i',j'}$ , and  $S_{J;i'',j''}^{i',j'}$ , respectively, where  $S_{L;i'',j''}^{i',j'}$ ,  $S_{G;i'',j''}^{i',j'}$ ,  $S_{K;i'',j''}^{i',j'}$ , and  $S_{J;i'',j''}^{i',j'}$  are the elements of  $\mathbf{S}_L^{i',j'}$ ,  $\mathbf{S}_G^{i',j'}$ ,  $\mathbf{S}_K^{i',j'}$ , and  $\mathbf{S}_J^{i',j'}$ , respectively, with  $(i'',j'')$  as their common subscripts.

Now we prove  $\mathbf{P}_M^{-\Delta_r^{(L)}(i'',j'')} = \mathbf{P}_M^{-\Delta_r^{(L)}(0,0)}$ .

$$\because 0 \leq i' \leq m-1, \therefore -m \leq -(m-i') \leq -1 \leq 0. \because M \geq m, \therefore 0 \leq M-m \leq M-(m-i') \leq M-1. \therefore \mathbf{P}_M^{-\Delta_r^{(L)}(0,0)} = \mathbf{P}_M^{-(M-(m-i'))}.$$

Now we split the set  $\{0, \dots, M-m\}$  into two parts,  $S_l = \{0, \dots, m-i'-1\}$  and  $S_t = \{m-i', \dots, M-m\}$ . If  $i'' \in S_l$ , then  $0 \leq i'' \leq m-i'-1$ .  $\therefore -M \leq -(m-i') \leq i'' - (m-i') \leq -1$ . In this case,  $\Delta_r^{(L)}(i'',j'') = (i'' - (m-i')) \bmod M - i'' = M + i'' - (m-i') - i'' = M - (m-i')$ . If  $i'' \in S_t$ , then  $m-i' \leq i'' \leq M-m$ .  $\therefore 0 \leq i'' - (m-i') \leq M-m - (m-i') < M$ . In this case,  $\Delta_r^{(L)}(i'',j'') = (i'' - (m-i')) \bmod M - i'' = i'' - (m-i') - i'' = -(m-i')$ .  $\therefore \mathbf{P}_M^{-(M-(m-i'))} = \mathbf{P}_M^{-i'}$ ,  $\therefore \mathbf{P}_M^{-\Delta_r^{(L)}(i'',j'')} = \mathbf{P}_M^{-(M-(m-i'))}$ ,  $\therefore \mathbf{P}_M^{-\Delta_r^{(L)}(i'',j'')} = \mathbf{P}_M^{-\Delta_r^{(L)}(0,0)}$ .

According to this proof, we also have  $\mathbf{P}_M^{-\Delta_r^{(G)}(i'',j'')} = \mathbf{P}_M^{-\Delta_r^{(G)}(0,0)}$ .

$$\text{Similarly, } \mathbf{Q}_N^{-\Delta_c^{(L)}(i'',j'')} = \mathbf{Q}_N^{-\Delta_c^{(L)}(0,0)} \text{ and } \mathbf{Q}_N^{-\Delta_c^{(K)}(i'',j'')} = \mathbf{Q}_N^{-\Delta_c^{(K)}(0,0)}.$$

Consequently, all increments in Eq.(4) are not related to  $(i'',j'')$ , and are constant, given  $(i',j')$ . All elements of  $\mathbf{S}^{L,i',j'}((M-m+i', N-n+j'), ((M-2m+i') \bmod M, (N-2n+j') \bmod N))$ ,

those of  $\mathbf{S}^{G,i',j'}((M-m+i',j'),((M-2m+i')\bmod M, N-n+j'))$ , those of  $\mathbf{S}^{K,i',j'}((i',N-n+j'),(M-m+i', (N-2n+j')\bmod N))$ , and those  $\mathbf{S}^{J,i',j'}((i',j'),(M-m+i', N-n+j'))$  are shifted with the same numbers of rows and columns, respectively. Noticed that  $d_L^{i',j'}(0,0)$ ,  $d_G^{i',j'}(0,0)$ ,  $d_K^{i',j'}(0,0)$ , and  $d_J^{i',j'}(0,0)$  are shifted to  $S_{L;0,0}^{i',j'}$ ,  $S_{G;0,0}^{i',j'}$ ,  $S_{K;0,0}^{i',j'}$ , and  $S_{J;0,0}^{i',j'}$ , respectively, therefore,

$$\begin{aligned} & \mathbf{S}_L^{i',j'}((0,0),(M-m-1,N-n-1)) \\ &= \mathbf{S}_L^{i',j'}((M-m+i',N-n+j'),((M-2m+i')\bmod M,(N-2n+j')\bmod N)), \\ & \mathbf{S}_G^{i',j'}((0,0),(M-m-1,N-n-1)) \\ &= \mathbf{S}_G^{i',j'}((M-m+i',j'),((M-2m+i')\bmod M,N-n+j')), \\ & \mathbf{S}_K^{i',j'}((0,0),(M-m-1,N-n-1)) \\ &= \mathbf{S}_K^{i',j'}((i',N-n+j'),(M-m+i',(N-2n+j')\bmod N)), \\ & \mathbf{S}_J^{i',j'}((0,0),(M-m-1,N-n-1)) \\ &= \mathbf{S}_J^{i',j'}((i',j'),(M-m+i',N-n+j')). \end{aligned}$$

Let  $\mathbf{C}^{i',j'} = \mathbf{S}_L^{i',j'} + \mathbf{S}_G^{i',j'} + \mathbf{S}_K^{i',j'} + \mathbf{S}_J^{i',j'}$ . Then, according to Eq.(3),  $C_{i'',j''}^{i',j'} = \mathbf{X}^{i',j'} \diamond \mathbf{Z}(i'',j'')$ .

Consequently, the correlation of  $\mathbf{X}^{i',j'}$  and  $\mathbf{Z}$ ,

$$\mathbf{X}^{i',j'} \diamond \mathbf{Z}(i'',j'') = \{C_{i'',j''}^{i',j'} | i'' = 0, \dots, M-m-1, j'' = 0, \dots, N-n-1\},$$

or briefly,

$$\mathbf{X}^{i',j'} \diamond \mathbf{Z} = \mathbf{C}^{i',j'}((0,0),(M-m-1,N-n-1)).$$

Q.E.D.

## 4 Other Experimental Results

We evaluate nBEKCF on VOT2016 dataset [8] which contains 60 sequences with substantial variations and challenges. We follow the VOT challenge protocol to compare trackers, where a tracker is re-initialized whenever its failure is observed. The evaluation criteria on VOT2016 are different from those on OTB-2013 and OTB-2015. On VOT2016, the accuracy and robustness of each tracker are evaluated in terms of the overlap ratios between bounding boxes and ground-truths and the number of re-initializations. In addition, VOT2016 mainly reports the expected average overlap (EAO) which integrates the accuracy and robustness of a tracker, and ranks trackers according to it, since the EAO score may provide an insight to the comprehensive performance of a tracker.

We compare our method against other top 9 trackers, SRDCF [2], DSST [1], NSAMF [8], deepMKCF [8], SAMF [7], KCF [6], ColorKCF [8], TGPR [4], and Struck [5], of VOT2016 challenge. Figs.3 shows the EAO ranking and accuracy-robustness plots, where the closer to the top-right corner of the plots a tracker is, the better the performance of the tracker is considered. It is seen that nBEKCF is ranked the second best in EAO. Although the EAO of nBEKCF is slightly less than that of SRDCF, it runs much faster than SRDCF (70fps vs. 7fps), and its memory requirement is much smaller than SRDCF's (130MB vs. 600MB), as shown in Table.1.

We also compare our nBEKCF and the above 9 trackers with the criteria used on OTB50 and OTB100. The results are shown in Fig.4. It is seen from the figure that nBEKCF outperforms the second best SRDCF on the average precision score and AUC by 2.0% and 2.1%, respectively. Table 2 shows the means of overlap precisions of all compared trackers, where our nBEKCF is also the best.

Table 1: Memory Requirement (MB) of Trackers.

| Tracker   | nBEKCF | SRDCF | DSST | KCF | NSAMF | SAMF | LCT | MEEM |
|-----------|--------|-------|------|-----|-------|------|-----|------|
| MemoryReq | 130    | 600   | 50   | 45  | 45    | 45   | 90  | 60   |

Table 2: Comparison of the 9 top trackers on the VOT2016 dataset in mean overlap precision. The best and second best results are shown in red and blue colors, respectively. Our nBEKCF achieves a gain of 4.71%, compared to the second best SRDCF.

| VOT2016 | nBEKCF        | ColorKCF | deepMKCF | DSST   | KCF    | NSAMF  | SAMF   | SRDCF         | Struck | TGPR   |
|---------|---------------|----------|----------|--------|--------|--------|--------|---------------|--------|--------|
| MeanOP  | <b>0.4812</b> | 0.3341   | 0.3840   | 0.3840 | 0.3315 | 0.3998 | 0.3642 | <b>0.4341</b> | 0.2337 | 0.2745 |

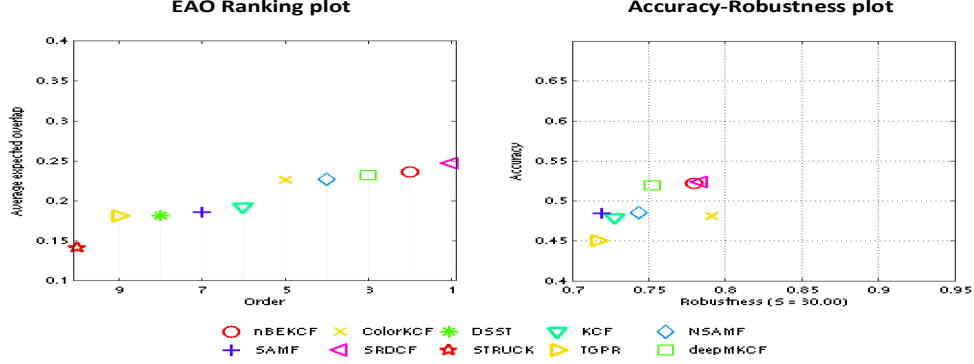

Figure 3: The EAO ranking and accuracy-robustness plots of nBEKCF, SRDCF [2], DSST [1], NSAMF [8], deepMKCF [8], SAMF [7], KCF [6], ColorKCF [8], TGPR [4], and Struck [5].

## References

- [1] M. Danelljan, G. Hager, F. Shahbaz Khan, and M. Felsberg. Accurate scale estimation for robust visual tracking. In *Proc. British Machine Vision Conference (BMVC)*, 2014.
- [2] M. Danelljan, G. Hager, F. Shahbaz Khan, and M. Felsberg. Learning spatially regularized correlation filters for visual tracking. In *Proc. International Conference on Computer Vision*, 2015.
- [3] P. David. *Circulant Matrices*. Chelsea Publishing Company, 2<sup>nd</sup> edition, 1994.
- [4] J. Gao, H. Ling, and J. Hu, W. and Xing. Transfer learning based visual tracking with gaussian process regression. In *Proc. European Conference on Computer Vision*, 2014.
- [5] S. Hare, A. Saffari, S. Golodetz, V. Vineet, M. Cheng, and P. Torr. Struck: Structured output tracking with kernels. *IEEE Transactions on Pattern Analysis and Machine Intelligence*, 2015.
- [6] J. Henriques, R. Caseiro, P. Martins, and J. Batista. High-speed tracking with kernelized correlation filters. *IEEE Transactions on Pattern Analysis and Machine Intelligence*, Vol.37:pp.583–596, 2015.
- [7] Y. Li and J. Zhu. A scale adaptive kernel correlation filter tracker with feature integration. In *Proc. European Conference on Computer Vision Workshop*, 2014.
- [8] M. Matej Kristan, A. Leonardis, J. Matas, M. Felsberg, and et. al. The visual object tracking vot2016 challenge results. In *Proc. Computer Vision - ECCV 2016 Workshops*, 2016.

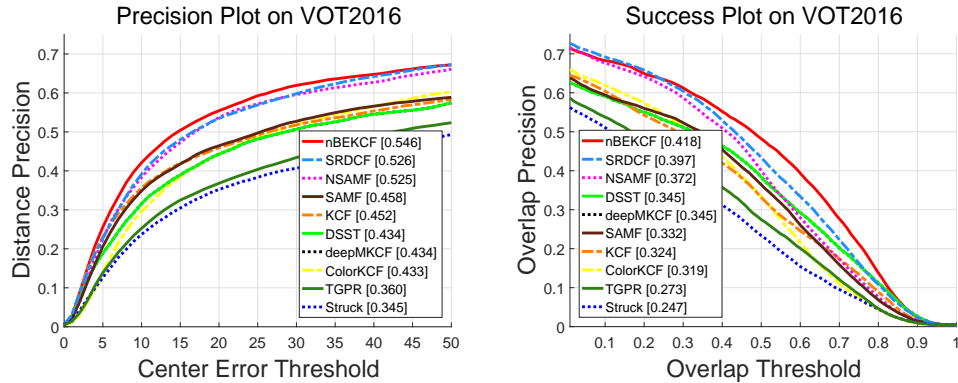

Figure 4: The precision and success plots of nBEKCF, SRDCF [2], DSST [1], NSAMF [8], deepMKCF [8], SAMF [7], KCF [6], ColorKCF [8], TGPR [4], and Struck [5].
